# Supplementary material for: Model Merging: Foundations and Algorithms
Source: arXiv:2605.01580 source file (2026-05-02)
Supplement: Supplementary file 2 [file fixed.tex]

%!TEX root = ../../../main.tex
\begin{algorithm}
    \caption{Fixed Merging Step}
    \label{alg:fixed-merging}
    \begin{algorithmic}[1]
      \REQUIRE Pretrained model weights $\theta_{\text{pre}}$, task-specific updates $\{\Delta_i\}_{i=1}^T$,
      user-specified threshold $\varepsilon$
      \ENSURE Fixed merged model weights 
      $\theta_{\text{MT}}$ 
      \\
   %\noindent  \hspace*{-\algorithmicindent}\hspace*{-\labelsep} 
   \STATE \textbf{Accounting for redundant directions} (\cref{sec:accounting_redundant})
      \STATE $\mathcal{M}=\{\}$ \label{line:start-discrad-directions}
      \FOR{$i=1,\dots,T$}
      \STATE $\delta_i \gets \text{vec}(\Delta_i)$ 
  \IF{
  $ \max_{\{j \in \mathcal{M}\}} \text{sim}(\delta_i, \delta_j) < \varepsilon$
  }
          \STATE $\mathcal{M} \gets \mathcal{M} \cup \{i\}$
        \ENDIF
      \ENDFOR \\ \label{line:end-discrad-directions}
 %\noindent   \hspace*{-\algorithmicindent}\hspace*{-\labelsep} 
 \STATE \textbf{Merging step using} \baseline{TSV-M} (\cref{ch:tsv}) \textbf{on the} $\{ \Delta_{i}\}_{i \in \mathcal{M}}$
      \FOR{$i \in \mathcal{M}$} \label{line:start-fixed_merging}
      \STATE $\Delta_i = U_i\,\Sigma_i\,V_i^\top$ 
      \STATE $\tilde{U}_i \gets U_{i{[:,1:k]}}$, $\tilde{\Sigma}_i \gets \Sigma_{i{[1:k,1:k]}}$, $\tilde{V}_i \gets V_{i{[:,1:k]}}$
      \ENDFOR
      %\STATE \textbf{Concatenate per-task subspaces}
      \STATE \quad $U \gets [\tilde{U}_1\,|\,\tilde{U}_2\,|\,\cdots\,|\,\tilde{U}_T]$
      \STATE \quad $\Sigma \gets \operatorname{block\_diag}(\tilde{\Sigma}_1,\tilde{\Sigma}_2,\dots,\tilde{\Sigma}_T)$
      \STATE \quad $V \gets [\tilde{V}_1\,|\,\tilde{V}_2\,|\,\cdots\,|\,\tilde{V}_T]$
      %\STATE \textbf{Orthogonalize to reduce inter-task interference}
      \STATE \quad  $U_\perp \gets \operatorname{orthogonalize}(U)$
      \STATE \quad  $V_\perp \gets \operatorname{orthogonalize}(V)$
      %\STATE \textbf{Compute fixed merging}
      \STATE \quad $\hat{\Delta} \gets U_\perp\,\Sigma\,V_\perp^\top$
    \STATE \quad  $\theta_{\text{MT}} \gets \theta_{\text{pre}} + \alpha\ \hat{\Delta}$ \label{line:end-fixed_merging}
       \STATE \textbf{return} $\theta_{\text{MT}}$ 
    \end{algorithmic}
  \end{algorithm}
